# Supplementary material for: On Gradient Coding with Partial Recovery
Source: arXiv:2102.10163 source file (2022-05-01)
Supplement: Supplementary file 1 [file Additional_Notes.tex]

$|\bigcup\limits_{j \in S} E_j|=|B|(1-\frac{{v-t \choose p}}{{v \choose p}})$ for every $S$ satisfying $|S|=n-s$.

Note that since the given assignment is a $t$-design, $|\bigcap\limits_{j \in S} E_j|=\lambda$. Also using the inclusion-exclusion principle for sets, we know that 

$$|\bigcup_{i\in [m]} C_i|= \sum_{i \in [m]} |C_i| - \sum_{1\leq i< j\leq m}|C_i\cap C_j|+\sum_{1\leq i< j<k\leq m}|C_i\cap C_j\cap C_k| + ..+(-1)^m|C_1\cap C_2\cap \ldots \cap C_m| $$

Note that in this case $C_i$ denote the set $E_i$ and $[m]$ denotes an possible subset $S$ with $|S|=n-s=t$. Now we know that $|C_1\cap C_2\cap \ldots \cap C_m|=\lambda$ and similarly $|C_{i_1}\cap C_{i_2} \cap \ldots \cap C_{i_a}|= \lambda \prod_{i=1}^{a} \frac{(v - t + i)}{(p - t + i)}$. Also, $\lambda=|B|\frac{{p \choose t}}{{v \choose t}}$ which can be shown on repeated application of the above result. 

Thus, the above expression evaluates to $|B|(\sum_{i=1}^{t} (-1)^i \frac{{p \choose i}}{{v \choose i}}. {{t \choose i}})= \frac{|B|}{{v \choose p}}(\sum_{i=1}^{t} (-1)^{i-1} {{v-i\choose v-p}}.{{t \choose i}})=|B|(1-\frac{{v-t \choose p}}{{v \choose p}})$.

\remove{Note that, the above expression can be computed using the idea of binomial expressions. Note that ${{k \choose i}}$ denotes the coefficient of $x^{i}$ in $(1+x)^k$ and $(-1)^i\times {{v-i\choose v-k}}$ denotes coefficient of $x^{(p-i)}$ in $(1+x)^{-(v-p+1)}$. Thus the numerator of the above expression is ${{v \choose p}}$ plus the coefficient of $x^p$ in $-(1+x)^t\times (1+x)^{-(v-p+1)}=-(1+x)^{-(v-p-t+1)}$ thus equals ${{v \choose p}}-{{v-t \choose p}}$. Hence, proved.}

%Thus, combining the fact that every $t$-design is a $u$-design for every $u \leq t$, we can show that $|\bigcup\limits_{j \in S} E_j|$ is fixed for every $S$ satisfying $|S|=n-s$

\remove{
\begin{lemma}
$|\bigcup\limits_{j \in S} E_j|={{v-t \choose k}}$ for every $|S|=t$
\end{lemma}
}

%%%%%%%%%%%%%%%%%%%%%%%%%%%%%%%%%%%%

We now derive a scheme based on the scheme proposed in Theorem \ref{high_comm_cyclic_middle_thm} which incurs a lower communication cost under the same computation load for a subset of parameters. {\color{red} Note that the inequality \eqref{high_comm_cyclic_middle_eqn2} is same as \eqref{high_comm_cyclic_middle_eqn1}.}

\remove{We now compute the number of data-partitions assigned to any of $n-s$ continuous workers whose indices are denoted by $I$.\remove{ We denote $J_i= \cup_{t \in I} {j:0\leq (t-j \mod n) \leq \gamma_i}$ for every $i \in [y]$ which denotes set of all possibilities for $i^{th}$ element in the list corresponding to the spanned data-partitions.} W.L.O.G, we assume that the indices of the non-straggled workers are $1,2,\ldots, n-s$. Consider all data-partitions not assigned to any of these workers whose $i^{th}$ element in the corresponding list is the largest, suppose we denote such a list by $\{c_1,c_2,\ldots c_y\}$. Thus, $c_i \leq (n-\gamma_i+1)$, $(c_{(j \mod n)+1)}-c_j) \geq \gamma_j$ for $j \in [y]$ and $c_{i+1}\geq n-s+1$. Thus, the number of such lists with the largest element being the $i^{th}$ element is given by ${{s-(\gamma_i)-\sum_{i=1}^{y-1}\gamma_i+y \choose y}}={{s-\delta+y \choose y}}$ as $\delta= \sum_{i=1}^{y}\gamma_i$. Thus, the total number of data-partitions not assigned to any of the consecutive $n-s$ workers is given by $y.{{s-\delta+y \choose y}}$. Thus, the number of gradients received at the master when consecutive $s$ workers straggle is given by $n.{{n-\delta+y-1 \choose y-1}}-y.{{s-\delta+y \choose y}}$.

\noindent {\bf Step 4: Lower bound on the number of data-partitions assigned to non-consecutive workers:} }

%%%%%%%%%%%%%%%%%%%%%%%%%%%%%%%%%%%%

\remove{
Note that for the case of $\gamma=1$, this parameter of this scheme is same as that of the scheme described in Sec ~\ref{compload_ub_section} where as for the case of $y=1$ it become same as that of the cyclic schemes as in Sec ~\ref{cyclic_scheme_section} except with a bit higher communication cost of $\gamma$ (transmitting all the data-partitions assigned). We denote $\gamma^{*}(y)$ as the minimum value of $\gamma$ satisfying the inequality \eqref{high_comm_cyclic_middle} for a given value of $y$. We can show that the computation load $\gamma^{*}(y).y$ typically decreases from the cyclic computation load in Sec ~\ref{cyclic_scheme_section} to Sec ~\ref{compload_ub_section} to as $y$ increases from 1 (stated as a corollary below) and the communication cost (as a function of $\gamma^{*}$ and $y$) decreases as $y$ increases from 1.

Thus, these give another set of gradient codes with computation load between the cyclic codes as discussed in Sec ~\ref{cyclic_scheme_section} and the optimal computation load as attained in Sec ~\ref{compload_ub_section}. Also note that the communication cost in this scheme typically lies between the two extremes.
}

Recall the assignment of data-partitions to workers described in the proof of Theorem~\ref{high_comm_cyclic_middle} where each data-partition is denoted by a list of size $y$ with integers $\{\gamma_i\}_{i=1}^{y}$ chosen satisfying $\sum_i{\gamma_i}=\delta$. We impose the additional constraint that $(c_{1+(i \mod n)}-c_i \mod n) \geq \gamma_i$ $\forall i \in [y]$. Note that corresponding to each such unique list, we had a unique data-partition. Now a data-partition denoted by the list ($[c_1,c_2,\ldots,c_y]$) is assigned to worker $W_j$ iff $0 \leq ((j - c_i) \mod n) \leq \gamma_i-1$ for some $i \in [y]$.

However, for the case of $\delta=y$ the communication cost of this scheme is $y$ times that of the one in Section ~\ref{compload_ub_section} whereas for the case of $y=1$, the communication cost is $\delta$(transmitting gradients of all the data-partitions assigned) unlike the scheme in Section ~\ref{cyclic_scheme_section} with communication cost of 1 or 2.

%%%%%%%%%%%%%%%%%%%%%%%%%%%%%%%%%%%%

\begin{figure}[ht]
\begin{minipage}[b]{0.45\linewidth}
\centering
\includegraphics[scale =0.5]{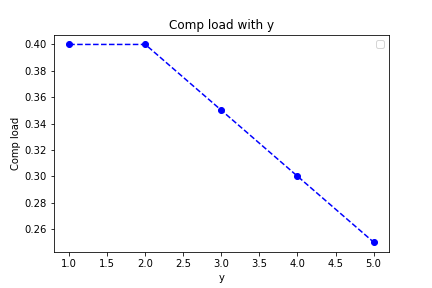}
\caption{Computation load with $y$ for $n=20$, $s=7$, $\alpha=0.998$}
\label{comp_load_n_20_s_7_alpha_998}
\end{minipage}
\hspace{0.5cm}
\begin{minipage}[b]{0.45\linewidth}
\centering
\includegraphics[scale = 0.5]{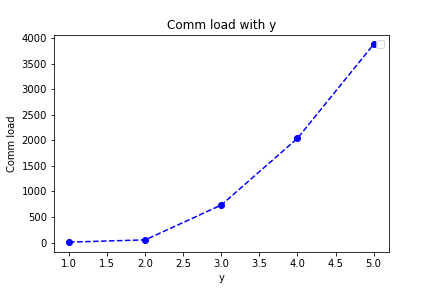}
\caption{Communication cost with $y$ for $n=20$, $s=7$, $\alpha=0.998$}
\label{comm_cost_n_20_s_7_alpha_998}
\end{minipage}
\end{figure}

%%%%%%%%%%%%%%%%%%%%%%%%%%%%%%%%%%%%

\begin{figure}[ht]
\begin{minipage}[b]{0.45\linewidth}
\centering
\includegraphics[scale =0.5]{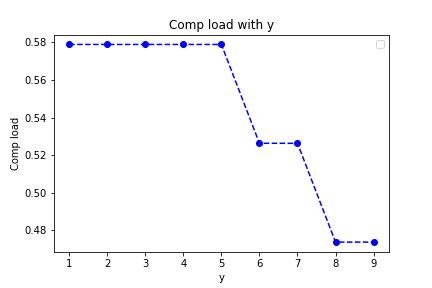}
\caption{Computation load with $y$ for $n=19$, $s=10$, $\alpha=0.9998$}
\label{comp_load_n_19_s_10_alpha_9998}
\end{minipage}
\hspace{0.5cm}
\begin{minipage}[b]{0.45\linewidth}
\centering
\includegraphics[scale = 0.5]{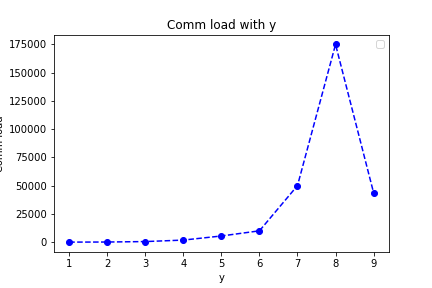}
\caption{Communication cost with $y$ for $n=19$, $s=10$, $\alpha=0.9998$}
\label{comm_cost_n_19_s_10_alpha_9998}
\end{minipage}
\end{figure}

Note that the values of $\delta^{*}(y)$ takes values $[11, 11, 11, 11, 11, 10, 10, 9, 9]$ for $y = [1,2,3,4,5,6,7,8,9]$ in Fig ~\ref{comp_load_n_19_s_10_alpha_9998},\ref{comm_cost_n_19_s_10_alpha_9998}. We plot the communication and computation cost according to Corollary ~\ref{high_comm_cyclic_middle_corollary}.
